# Supplementary material for: Covariant BSSN formulation in bimetric relativity
Source: arXiv:1904.07869 ancillary file (2020-03-06)
Supplement: Supplementary file 1 [file Addendum-lapse-ratio.pdf]

# Supplementary material to:
# Covariant BSSN formulation in bimetric relativity

**Francesco Torsello, Mikica Kocic, Marcus Högås, Edvard Mörtsell**

*Department of Physics & The Oskar Klein Centre,*
*Stockholm University, AlbaNova University Center, SE-106 91 Stockholm, Sweden*

*E-mail:* `francesco.torsello@fysik.su.se`

## Contents

1 The ratio of the lapses in the spherically symmetric covariant BSSN formulation 1

# 1 The ratio of the lapses in the spherically symmetric covariant BSSN formulation

In this addendum, we write the ratio of the lapses $W$ for the ansatz (A.50) in the main paper. In [1], $W$ is computed for the spherically symmetric standard $3+1$ formulation. Here we recast it in the spherically symmetric cBSSN formulation and write it using a color code to highlight its structure. Blue refers to the $g$-sector, red to the $f$-sector, orange to the Lorentz frame, magenta to the interaction terms. We have,

$$\frac{\alpha}{\tilde{\alpha}} = -\frac{W_f}{W_g} =: W, \tag{1.1}$$

where

$$\begin{aligned} W_g =\ & \lambda^2\big[c_1 + \lambda(c_2 + \lambda c_3) + \mathbf{p}^{12}c_4\big] + \kappa_f\lambda^2(c_5 + \lambda c_6) \\ & + \kappa_g\lambda^2\big[c_7 + \lambda^2 c_9 + \lambda(c_8 + \mathbf{p}^{1}c_{10}) + \mathbf{p}^{12}c_{11}\big] \\ & + \mathbf{p}^{1}\lambda\big[c_{12} + \lambda(c_{13} + \lambda c_{14}) + \mathbf{p}^{12}c_{15}\big]e^{2\psi}\big(2\,\widehat{b}\,\partial_r\psi + \partial_r\widehat{b}\big) \\ & + \lambda^2(c_{16} + \lambda c_{17})e^{4\psi}\big(2\,\widehat{b}\,\partial_r\psi + \partial_r\widehat{b}\big)^2 \\ & + \big[\mathbf{p}^{1}\lambda^2(c_{18} + \lambda c_{19}) + \lambda^3(c_{20} + \lambda c_{21})e^{2\psi}\big(2\,\widehat{b}\,\partial_r\psi + \partial_r\widehat{b}\big)\big]e^{2\phi}\big(2\,\overline{b}\,\partial_r\phi + \partial_r\overline{b}\big) \\ & + \lambda^2\big[\lambda(c_{22} + \lambda c_{23}) + \mathbf{p}^{12}c_{24}\big]e^{4\phi}\big(2\,\overline{b}\,\partial_r\phi + \partial_r\overline{b}\big)^2, \end{aligned} \tag{1.2a}$$

$$\begin{aligned} W_f =\ & \lambda^2\big[d_1 + \lambda(d_2 + \lambda d_3) + \mathbf{p}^{12}d_4\big] + \kappa_f\lambda^2\big[d_5 + \lambda^2 d_7 + \lambda(d_6 + \mathbf{p}^{1}d_8) + \mathbf{p}^{12}d_9\big] \\ & + \kappa_g\lambda^2(d_{10} + \lambda d_{11}) + \mathbf{p}^{1}\lambda^2(d_{12} + \lambda d_{13})e^{2\psi}\big(2\,\widehat{b}\,\partial_r\psi + \partial_r\widehat{b}\big) \\ & + \lambda^2\big[\lambda(d_{14} + \lambda d_{15}) + \mathbf{p}^{12}d_{16}\big]e^{4\psi}\big(2\,\widehat{b}\,\partial_r\psi + \partial_r\widehat{b}\big)^2 \\ & + \Big\{\mathbf{p}^{1}\lambda\big[d_{17} + \lambda(d_{18} + \lambda d_{19}) + \mathbf{p}^{12}d_{20}\big] + \lambda^3(d_{21} + \lambda d_{22})e^{2\psi}\big(2\,\widehat{b}\,\partial_r\psi + \partial_r\widehat{b}\big)\Big\}\cdot \\ & \cdot e^{2\phi}\big(2\,\overline{b}\,\partial_r\phi + \partial_r\overline{b}\big) + \lambda^2(d_{23} + \lambda d_{24})e^{4\phi}\big(2\,\overline{b}\,\partial_r\phi + \partial_r\overline{b}\big)^2. \end{aligned} \tag{1.2b}$$

The coefficients $c_i$ are given below,

$$\begin{aligned} c_1 =\ & 2e^{6\psi+4\phi}\widehat{a}^3\overline{a}^2\widehat{R}\Big[\Big(\big\langle\widehat{R}\big\rangle_1^1\Big)^2 - \widehat{R}^2\Big(\big\langle\widehat{R}\big\rangle_2^1\Big)^2 \\ & + e^{4\phi}\overline{b}^2\widehat{R}^2\Big(\widehat{A}_2 + \tfrac{\widehat{K}}{3}\Big)^2\big\langle\widehat{R}\big\rangle_1^1\Big(4\big\langle\widehat{R}\big\rangle_1^1 - 3\big\langle\widehat{R}\big\rangle_1^2\Big)\Big], \end{aligned} \tag{1.3a}$$

$$c_2 = 2e^{4\psi+6\phi}\widehat{a}^2\overline{a}^2\widehat{R}^2\Bigg\{\overline{a}\Big[\Big\{-1 - e^{4\phi}\overline{b}^2\Big[4\widehat{R}^2\Big(\widehat{A}_2 + \tfrac{\widehat{K}}{3}\Big)^2 + 3\Big(\overline{A}_2 + \tfrac{\overline{K}}{3}\Big)^2\Big]\Big\}\Big(\big\langle\widehat{R}\big\rangle_1^1\Big)^2$$

$$
\begin{aligned}
&+\widehat{R}\left\langle\widehat{R}\right\rangle_2^1\cdot\\
&\cdot\left[\widehat{R}\left\langle\widehat{R}\right\rangle_2^1+e^{4\phi}\bar{b}^2\left(\bar{A}_2+\frac{\bar{K}}{3}\right)^2\left(\widehat{R}\left\langle\widehat{R}\right\rangle_2^1-2\beta_{(1)}\right)\right]+2e^{4\phi}\bar{b}^2\widehat{R}\left(\bar{A}_2+\frac{\bar{K}}{3}\right)^2\left\langle\widehat{R}\right\rangle_1^1\beta_{(2)}\Bigg]\\
&+2e^{2(\psi+\phi)}\hat{a}\bar{b}^2\widehat{R}\left(\widehat{A}_2+\frac{\widehat{K}}{3}\right)\left(\bar{A}_2+\frac{\bar{K}}{3}\right)\left[-\left\langle\widehat{R}\right\rangle_2^1\beta_{(1)}-\left\langle\widehat{R}\right\rangle_1^1\left(2\beta_{(2)}+3\widehat{R}\beta_{(3)}\right)\right]\Bigg\},
\end{aligned}
\tag{1.3b}
$$

$$
\begin{aligned}
c_3 =& -2e^{4\psi+8\phi}\hat{a}^2\bar{a}^2\bar{b}^2\left(\bar{A}_2+\frac{\bar{K}}{3}\right)\cdot\\
&\cdot\Bigg\{2e^{2\phi}\bar{a}\widehat{R}^2\left(\widehat{A}_2+\frac{\widehat{K}}{3}\right)\left[-4\left\langle\widehat{R}\right\rangle_1^1\left\langle\widehat{R}\right\rangle_0^2+\left\langle\widehat{R}\right\rangle_0^1\left(4\left\langle\widehat{R}\right\rangle_1^1+\left\langle\widehat{R}\right\rangle_1^2\right)+\left\langle\widehat{R}\right\rangle_1^2\beta_{(0)}\right]\\
&+e^{2\psi}\hat{a}\left(\bar{A}_2+\frac{\bar{K}}{3}\right)\left[-4\left\langle\widehat{R}\right\rangle_1^1\left\langle\widehat{R}\right\rangle_0^2+\left\langle\widehat{R}\right\rangle_0^1\left(4\left\langle\widehat{R}\right\rangle_1^1+\left\langle\widehat{R}\right\rangle_1^2\right)+\left\langle\widehat{R}\right\rangle_1^2(\left\langle\widehat{R}\right\rangle_0^2\\
&\qquad+\widehat{R}\left\langle\widehat{R}\right\rangle_1^2+2\beta_{(0)})\right]\Bigg\},
\end{aligned}
\tag{1.3c}
$$

$$
c_4 = -2e^{6\psi+8\phi}\hat{a}^3\bar{a}^2\bar{b}^2\widehat{R}^2\left(\bar{A}_2+\frac{\bar{K}}{3}\right)^2\left\langle\widehat{R}\right\rangle_2^1(4\left\langle\widehat{R}\right\rangle_1^1-\left\langle\widehat{R}\right\rangle_1^2), \tag{1.3d}
$$

$$
c_5 = -e^{6\psi+8\phi}\hat{a}^3\bar{a}^2\bar{b}^2\left\langle\widehat{R}\right\rangle_1^2\left[\left(\left\langle\widehat{R}\right\rangle_1^1\right)^2-3\widehat{R}^2\left(\left\langle\widehat{R}\right\rangle_2^1\right)^2-2\widehat{R}\left\langle\widehat{R}\right\rangle_1^1\left(\left\langle\widehat{R}\right\rangle_2^1+\left\langle\widehat{R}\right\rangle_2^2-\tilde{\rho}^{\mathrm{m}}\widehat{R}^2\right)\right], \tag{1.3e}
$$

$$
c_6 = 6e^{4\psi+10\phi}\hat{a}^2\bar{a}^3\bar{b}^2\left(-\left\langle\widehat{R}\right\rangle_0^1+\left\langle\widehat{R}\right\rangle_0^2\right)\left(\left\langle\widehat{R}\right\rangle_1^2\right)^2, \tag{1.3f}
$$

$$
c_7 = e^{6\psi+8\phi}\hat{a}^3\bar{a}^2\bar{b}^2\widehat{R}^2\left\langle\widehat{R}\right\rangle_1^2\left[-2\left\langle\widehat{R}\right\rangle_2^1\left\langle\widehat{R}\right\rangle_0^2+\left\langle\widehat{R}\right\rangle_1^2\left(-4\left\langle\widehat{R}\right\rangle_1^1+\left\langle\widehat{R}\right\rangle_1^2\right)\right], \tag{1.3g}
$$

$$
\begin{aligned}
c_8 =& -2e^{4\psi+10\phi}\hat{a}^2\bar{a}^3\bar{b}^2\widehat{R}^2\left\langle\widehat{R}\right\rangle_1^2\cdot\\
&\cdot\left[2\left\langle\widehat{R}\right\rangle_1^1\left(-J^{\mathrm{m}\theta}{}_\theta+\left\langle\widehat{R}\right\rangle_0^2\right)+\left(-J^{\mathrm{m}r}{}_r+\rho^{\mathrm{m}}+\left\langle\widehat{R}\right\rangle_0^1-\left\langle\widehat{R}\right\rangle_0^2\right)\left\langle\widehat{R}\right\rangle_1^2\right],
\end{aligned}
\tag{1.3h}
$$

$$
c_9 = 2e^{6\psi+8\phi}\hat{a}^3(2J^{\mathrm{m}\theta}{}_\theta-\rho^{\mathrm{m}})\bar{a}^2\bar{b}^2\widehat{R}^2\left\langle\widehat{R}\right\rangle_2^1\left\langle\widehat{R}\right\rangle_1^2, \tag{1.3i}
$$

$$
c_{10} = 4e^{6(\psi+\phi)}\hat{a}^3 j^{\mathrm{m}}\bar{a}\bar{b}^2\widehat{R}^2\left\langle\widehat{R}\right\rangle_2^1\left\langle\widehat{R}\right\rangle_1^2, \tag{1.3j}
$$

$$
c_{11} = -2e^{6\psi+8\phi}\hat{a}^3\rho^{\mathrm{m}}\bar{a}^2\bar{b}^2\widehat{R}^2\left\langle\widehat{R}\right\rangle_2^1\left\langle\widehat{R}\right\rangle_1^2, \tag{1.3k}
$$

$$
c_{12} = 8e^{2\psi+8\phi}\hat{a}\bar{a}^3\bar{b}\widehat{R}^2\left(\bar{A}_2+\frac{\bar{K}}{3}\right)\left(\left\langle\widehat{R}\right\rangle_1^1\right)^2, \tag{1.3l}
$$

$$
c_{13} = 4e^{4\psi+6\phi}\hat{a}^2\bar{a}^2\bar{b}\widehat{R}^2\left(\bar{A}_2+\frac{\bar{K}}{3}\right)\left[\left\langle\widehat{R}\right\rangle_2^1\beta_{(1)}+\left\langle\widehat{R}\right\rangle_1^1\left(2\beta_{(2)}+3\widehat{R}\beta_{(3)}\right)\right], \tag{1.3m}
$$

$$
c_{14} = -4e^{2\psi+8\phi}\hat{a}\bar{a}^3\bar{b}\widehat{R}^2\left(\bar{A}_2+\frac{\bar{K}}{3}\right)\left[2\widehat{R}\left\langle\widehat{R}\right\rangle_1^1\beta_{(2)}+\beta_{(1)}(-\beta_{(1)}+\widehat{R}^2\beta_{(3)})\right], \tag{1.3n}
$$

$$
c_{15} = 8e^{2\psi+8\phi}\hat{a}\bar{a}^3\bar{b}\widehat{R}^2\left(\bar{A}_2+\frac{\bar{K}}{3}\right)\left(\left\langle\widehat{R}\right\rangle_1^1\right)^2, \tag{1.3o}
$$

$$
c_{16} = -2e^{2\psi+4\phi}\hat{a}\bar{a}^2\widehat{R}\left\{\beta_{(1)}^2+\widehat{R}\left[5\beta_{(1)}\beta_{(2)}+\widehat{R}\left(2\beta_{(2)}^2+5\beta_{(1)}\beta_{(3)}+3\widehat{R}\beta_{(2)}\beta_{(3)}\right)\right]\right\}, \tag{1.3p}
$$

$$
c_{17} = 8e^{6\phi}\bar{a}^3\widehat{R}^2\left(\left\langle\widehat{R}\right\rangle_1^1\right)^2, \tag{1.3q}
$$

$$
c_{18} = 4e^{6\psi+4\phi}\hat{a}^3\bar{a}\bar{b}\widehat{R}^3\left(\widehat{A}_2+\frac{\widehat{K}}{3}\right)\left[\left\langle\widehat{R}\right\rangle_2^1\beta_{(1)}+\left\langle\widehat{R}\right\rangle_1^1\left(2\beta_{(2)}+3\widehat{R}\beta_{(3)}\right)\right], \tag{1.3r}
$$

$$
c_{19} = 4e^{4(\psi+\phi)}\hat{a}^2\bar{a}\bar{b}\widehat{R}^2\cdot
$$

$$\cdot \Big\{e^{2\phi}\bar{a}\Big(\hat{A}_2+\tfrac{\hat{K}}{3}\Big)\Big[-4\left\langle\hat{R}\right\rangle_1^1\left\langle\hat{R}\right\rangle_0^2+\left\langle\hat{R}\right\rangle_0^1\Big(4\left\langle\hat{R}\right\rangle_1^1+\left\langle\hat{R}\right\rangle_1^2\Big)+\left\langle\hat{R}\right\rangle_1^2\beta_{(0)}\Big]$$

$$+\,2e^{2\psi}\hat{a}\Big(\bar{A}_2+\tfrac{\bar{K}}{3}\Big)\Big[\beta_{(1)}\beta_{(2)}+\left\langle\hat{R}\right\rangle_1^1\Big(3\left\langle\hat{R}\right\rangle_2^1+\beta_{(2)}\Big)-\Big(\left\langle\hat{R}\right\rangle_0^1+\beta_{(0)}\Big)\beta_{(3)}\Big]\Big\}, \quad (1.3s)$$

$$c_{20}=4e^{4\psi+2\phi}\hat{a}^2\bar{a}\hat{R}^2\Big\{3\beta_{(1)}\beta_{(2)}+\hat{R}\Big[2(\beta_{(2)})^2+\Big(-3\left\langle\hat{R}\right\rangle_1^1+\beta_{(1)}\Big)\beta_{(3)}\Big]\Big\}, \quad (1.3t)$$

$$c_{21}=4e^{2\psi+4\phi}\hat{a}\bar{a}^2\hat{R}^2\Big[-3\beta_{(1)}^2-6\hat{R}\beta_{(1)}\beta_{(2)}+\hat{R}^2\left(-4\beta_{(2)}^2+\beta_{(1)}\beta_{(3)}\right)\Big], \quad (1.3u)$$

$$c_{22}=-2e^{4\psi+2\phi}\hat{a}^2\bar{a}\hat{R}^2\Big\{-3\beta_{(1)}^2+\hat{R}\Big[-6\beta_{(1)}\beta_{(2)}+\hat{R}\Big(\left\langle\hat{R}\right\rangle_2^1\left\langle\hat{R}\right\rangle_2^1-5\beta_{(2)}^2+2\beta_{(1)}\beta_{(3)}\Big)\Big]\Big\}, \quad (1.3v)$$

$$c_{23}=-2e^{6\psi}\hat{a}^3\hat{R}^2\left\langle\hat{R}\right\rangle_2^1\Big(4\left\langle\hat{R}\right\rangle_1^1-\left\langle\hat{R}\right\rangle_1^2\Big), \quad (1.3w)$$

$$c_{24}=-2e^{6\psi}\hat{a}^3\hat{R}^2\Big[\beta_{(1)}\beta_{(2)}+\hat{R}^3\beta_{(3)}^2-\left\langle\hat{R}\right\rangle_1^1\left(2\beta_{(2)}+5\hat{R}\beta_{(3)}\right)\Big]. \quad (1.3x)$$

The coefficients $d_i$ are,

$$d_1=2e^{4\psi+6\phi}\hat{a}^2\bar{a}^3\hat{R}^2\left\langle\hat{R}\right\rangle_2^1\cdot$$

$$\cdot\Big[-e^{4\phi}\bar{b}^2\Big(\bar{A}_2+\tfrac{\bar{K}}{3}\Big)^2\Big(-4\left\langle\hat{R}\right\rangle_1^1+\left\langle\hat{R}\right\rangle_1^2\Big)+\beta_{(1)}+\hat{R}\Big(-\left\langle\hat{R}\right\rangle_2^1+\beta_{(2)}\Big)\Big], \quad (1.4a)$$

$$d_2=2e^{4(\psi+\phi)}\hat{a}^2\bar{a}^2\Big\{e^{2\psi}\hat{a}\Big[\Big(-1+e^{4\phi}\bar{b}^2\hat{R}^2\Big(\hat{A}_2+\tfrac{\hat{K}}{3}\Big)^2\Big)\Big(\left\langle\hat{R}\right\rangle_1^1\Big)^2$$

$$+\,\hat{R}^2\left\langle\hat{R}\right\rangle_2^1\Big\{\left\langle\hat{R}\right\rangle_2^1+e^{4\phi}\bar{b}^2\Big[4\Big(\bar{A}_2+\tfrac{\bar{K}}{3}\Big)^2\left\langle\hat{R}\right\rangle_2^1+\Big(\hat{A}_2+\tfrac{\hat{K}}{3}\Big)^2\Big(\left\langle\hat{R}\right\rangle_0^1-3\left\langle\hat{R}\right\rangle_0^2$$

$$+\,3\hat{R}\left\langle\hat{R}\right\rangle_1^2-2\beta_{(0)}\Big)\Big]\Big\}-2e^{4\phi}\bar{b}^2\hat{R}\Big(\hat{A}_2+\tfrac{\hat{K}}{3}\Big)^2\left\langle\hat{R}\right\rangle_1^1\Big(\left\langle\hat{R}\right\rangle_0^1+\beta_{(0)}\Big)\Big]$$

$$+\,2e^{6\phi}\bar{a}\bar{b}^2\hat{R}^3\Big(\hat{A}_2+\tfrac{\hat{K}}{3}\Big)\Big(\bar{A}_2+\tfrac{\bar{K}}{3}\Big)\Big[\left\langle\hat{R}\right\rangle_2^1\beta_{(1)}+\left\langle\hat{R}\right\rangle_1^1\left(2\beta_{(2)}+3\hat{R}\beta_{(3)}\right)\Big]\Big\}, \quad (1.4b)$$

$$d_3=2e^{4\psi+6\phi}\hat{a}^2\bar{a}^2\hat{R}\Big\{\bar{a}\left\langle\hat{R}\right\rangle_1^1\left\langle\hat{R}\right\rangle_1^2$$

$$+\,e^{4\phi}\bar{a}\bar{b}^2\hat{R}^2\Big(\hat{A}_2+\tfrac{\hat{K}}{3}\Big)^2\Big[\Big(\left\langle\hat{R}\right\rangle_1^1\Big)^2+2\hat{R}^2\left\langle\hat{R}\right\rangle_2^1\beta_{(2)}+\hat{R}\left\langle\hat{R}\right\rangle_1^1\Big(5\left\langle\hat{R}\right\rangle_2^1+2\beta_{(2)}\Big)\Big]$$

$$-\,2e^{2(\psi+\phi)}\hat{a}\bar{b}^2\hat{R}^2\Big(\hat{A}_2+\tfrac{\hat{K}}{3}\Big)\Big(\bar{A}_2+\tfrac{\bar{K}}{3}\Big)\Big[3\Big(\left\langle\hat{R}\right\rangle_2^1\Big)^2+\beta_{(2)}^2-\beta_{(1)}\beta_{(3)}\Big]\Big\}, \quad (1.4c)$$

$$d_4=2e^{4\psi+6\phi}\hat{a}^2\bar{a}^3\hat{R}\left\langle\hat{R}\right\rangle_1^1\Big[-\left\langle\hat{R}\right\rangle_1^2+e^{4\phi}\bar{b}^2\hat{R}^2\Big(\hat{A}_2+\tfrac{\hat{K}}{3}\Big)^2\Big(-4\left\langle\hat{R}\right\rangle_1^1+3\left\langle\hat{R}\right\rangle_1^2\Big)\Big], \quad (1.4d)$$

$$d_5=e^{4\psi+10\phi}\hat{a}^2\bar{a}^3\bar{b}^2\Big(\left\langle\hat{R}\right\rangle_1^2\Big)^2\Big(-4\left\langle\hat{R}\right\rangle_1^1+3\left\langle\hat{R}\right\rangle_1^2\Big), \quad (1.4e)$$

$$d_6=-2e^{6\psi+8\phi}\hat{a}^3\bar{a}^2\bar{b}^2\left\langle\hat{R}\right\rangle_1^2\Big\{\left\langle\hat{R}\right\rangle_1^1\Big[\Big(\tilde{J}^{\mathrm{m}\,r}{}_r-\tilde{\rho}^{\mathrm{m}}\Big)\hat{R}^2+\left\langle\hat{R}\right\rangle_2^1\Big]$$

$$+\,\hat{R}\left\langle\hat{R}\right\rangle_2^1\Big[\Big(\tilde{J}^{\mathrm{m}\,r}{}_r+2\tilde{J}^{\mathrm{m}\,\theta}{}_\theta-\tilde{\rho}^{\mathrm{m}}\Big)\hat{R}^2+\left\langle\hat{R}\right\rangle_2^1-2\left\langle\hat{R}\right\rangle_2^2\Big]\Big\}, \quad (1.4f)$$

$$d_7=-2e^{4\psi+10\phi}\hat{a}^2\bar{a}^3\bar{b}^2\Big(\left\langle\hat{R}\right\rangle_0^1-\left\langle\hat{R}\right\rangle_0^2\Big)\left\langle\hat{R}\right\rangle_1^2\Big[\Big(-2\tilde{J}^{\mathrm{m}\,\theta}{}_\theta+\tilde{\rho}^{\mathrm{m}}\Big)\hat{R}^2+\left\langle\hat{R}\right\rangle_2^2\Big], \quad (1.4g)$$

$$d_8=4e^{2(\psi+5\phi)}\tilde{J}^{\mathrm{m}}\hat{a}\bar{a}^3\bar{b}^2\hat{R}^2\Big(-\left\langle\hat{R}\right\rangle_0^1+\left\langle\hat{R}\right\rangle_0^2\Big)\left\langle\hat{R}\right\rangle_1^2, \quad (1.4h)$$

$$d_9=2e^{4\psi+10\phi}\hat{a}^2\bar{a}^3\bar{b}^2\Big(\left\langle\hat{R}\right\rangle_0^1-\left\langle\hat{R}\right\rangle_0^2\Big)\left\langle\hat{R}\right\rangle_1^2\Big(-\tilde{\rho}^{\mathrm{m}}\hat{R}^2+\left\langle\hat{R}\right\rangle_2^2\Big), \quad (1.4i)$$

$$d_{10}=e^{4\psi+10\phi}\hat{a}^2\bar{a}^3\bar{b}^2\hat{R}^2\left\langle\hat{R}\right\rangle_1^2\Big[2\left\langle\hat{R}\right\rangle_2^1\Big(\rho^{\mathrm{m}}-\left\langle\hat{R}\right\rangle_0^2\Big)-4\left\langle\hat{R}\right\rangle_1^1\left\langle\hat{R}\right\rangle_1^2+\Big(\left\langle\hat{R}\right\rangle_1^2\Big)^2\Big], \quad (1.4j)$$

$$d_{11} = -6e^{6\psi+8\phi}\hat{a}^3\bar{a}^2\bar{b}^2\widehat{R}^2\left\langle\widehat{R}\right\rangle_2^1\left(\left\langle\widehat{R}\right\rangle_1^2\right)^2, \tag{1.4k}$$

$$d_{12} = 4e^{2\psi+8\phi}\hat{a}\bar{a}^3\bar{b}\widehat{R}^2\left(\bar{A}_2 + \frac{\bar{K}}{3}\right)\left[\left\langle\widehat{R}\right\rangle_2^1\beta_{(1)} + \left\langle\widehat{R}\right\rangle_1^1\left(2\beta_{(2)} + 3\widehat{R}\beta_{(3)}\right)\right], \tag{1.4l}$$

$$\begin{aligned} d_{13} = 4e^{2\psi+6\phi}\hat{a}\bar{a}^2\bar{b}\widehat{R}^2\Big\{&-e^{2\psi}\hat{a}\left(\bar{A}_2 + \frac{\bar{K}}{3}\right)\left[3\left(\left\langle\widehat{R}\right\rangle_2^1\right)^2 + \beta_{(2)}^2 - \beta_{(1)}\beta_{(3)}\right] \\ &- 2e^{2\phi}\bar{a}\widehat{R}\left(\widehat{A}_2 + \frac{\widehat{K}}{3}\right)\left[\left\langle\widehat{R}\right\rangle_2^1\beta_{(1)} + \left\langle\widehat{R}\right\rangle_1^1\left(2\beta_{(2)} + 3\widehat{R}\beta_{(3)}\right)\right]\Big\}, \end{aligned} \tag{1.4m}$$

$$d_{14} = 2e^{2\psi+4\phi}\hat{a}\bar{a}^2\left[\beta_{(1)}^2 + \widehat{R}\left\{2\beta_{(1)}\beta_{(2)} - \widehat{R}\left[3\left(\left\langle\widehat{R}\right\rangle_2^1\right)^2 + \beta_{(2)}^2 - 2\beta_{(1)}\beta_{(3)}\right]\right\}\right], \tag{1.4n}$$

$$d_{15} = 2e^{6\phi}\bar{a}^3\widehat{R}\left\langle\widehat{R}\right\rangle_1^1\left(-4\left\langle\widehat{R}\right\rangle_1^1 + 3\left\langle\widehat{R}\right\rangle_1^2\right), \tag{1.4o}$$

$$d_{16} = 2e^{6\phi}\bar{a}^3\widehat{R}\left\{\beta_{(1)}^2 + \widehat{R}\left[5\beta_{(1)}\beta_{(2)} + \widehat{R}\left(2\beta_{(2)}^2 + 5\beta_{(1)}\beta_{(3)} + 3\widehat{R}\beta_{(2)}\beta_{(3)}\right)\right]\right\}, \tag{1.4p}$$

$$d_{17} = -8e^{6\psi+4\phi}\hat{a}^3\bar{a}\bar{b}\widehat{R}^2\left(\widehat{A}_2 + \frac{\widehat{K}}{3}\right)\left\langle\widehat{R}\right\rangle_2^1\left\langle\widehat{R}\right\rangle_1^2, \tag{1.4q}$$

$$d_{18} = 4e^{4\psi+6\phi}\hat{a}^2\bar{a}^2\bar{b}\widehat{R}^3\left(\widehat{A}_2 + \frac{\widehat{K}}{3}\right)\left[\left\langle\widehat{R}\right\rangle_2^1\beta_{(1)} + \left\langle\widehat{R}\right\rangle_1^1\left(2\beta_{(2)} + 3\widehat{R}\beta_{(3)}\right)\right], \tag{1.4r}$$

$$\begin{aligned} d_{19} = {} & 4e^{6\psi+4\phi}\hat{a}^3\bar{a}\bar{b}\widehat{R}^2\left(\widehat{A}_2 + \frac{\widehat{K}}{3}\right)\cdot \\ & \cdot\left\{2\beta_{(1)}\beta_{(2)} + \widehat{R}\left[8\beta_{(2)}^2 + \beta_{(1)}\beta_{(3)} + \widehat{R}\beta_{(3)}\left(12\beta_{(2)} + 5\widehat{R}\beta_{(3)}\right)\right]\right\}, \end{aligned} \tag{1.4s}$$

$$d_{20} = -8e^{6\psi+4\phi}\hat{a}^3\bar{a}\bar{b}\widehat{R}^2\left(\widehat{A}_2 + \frac{\widehat{K}}{3}\right)\left\langle\widehat{R}\right\rangle_2^1\left\langle\widehat{R}\right\rangle_1^2, \tag{1.4t}$$

$$d_{21} = -4e^{2\psi+4\phi}\hat{a}\bar{a}^2\widehat{R}^2\left\{3\beta_{(1)}\beta_{(2)} + \widehat{R}\left[2\beta_{(2)}^2 + \left(-3\left\langle\widehat{R}\right\rangle_1^1 + \beta_{(1)}\right)\beta_{(3)}\right]\right\}, \tag{1.4u}$$

$$d_{22} = 4e^{4\psi+2\phi}\hat{a}^2\bar{a}\widehat{R}^2\left[3\left(\left\langle\widehat{R}\right\rangle_2^1\right)^2 + \beta_{(2)}^2 - \beta_{(1)}\beta_{(3)}\right], \tag{1.4v}$$

$$d_{23} = 2e^{4\psi+2\phi}\hat{a}^2\bar{a}\widehat{R}^2\left[\beta_{(1)}\beta_{(2)} + \widehat{R}^3\beta_{(3)}^2 - \left\langle\widehat{R}\right\rangle_1^1\left(2\beta_{(2)} + 5\widehat{R}\beta_{(3)}\right)\right], \tag{1.4w}$$

$$d_{24} = -8e^{6\psi}\hat{a}^3\widehat{R}^2\left(\left\langle\widehat{R}\right\rangle_2^1\right)^2. \tag{1.4x}$$

## References


[1] M. Kocic, A. Lundkvist and F. Torsello, *On the ratio of lapses in bimetric relativity*, *Classical and Quantum Gravity* **36** (oct, 2019) 225013.
